# Supplementary material for: Carbon, nitrogen and oxygen abundance gradients in M101 and M31
Source: arXiv:1911.01981 source file (2019-11-05)
Supplement: Supplementary file 1 [file Supplemental_Appendix.pdf]

MNRAS 000, 1–1 (2019) Preprint 29 October 2019 Compiled using MNRAS LaTeX style file v3.0

# Appendix: Carbon, nitrogen and oxygen abundance gradients in M101 and M31

C. Esteban,[1,2]★ F. Bresolin,[3] J. García-Rojas,[1,2] and L. Toribio San Cipriano[1,2]
[1]*Instituto de Astrofísica de Canarias, E-38200 La Laguna, Tenerife, Spain*
[2]*Departamento de Astrofísica, Universidad de La Laguna, E-38206, La Laguna, Tenerife, Spain*
[3]*Institute for Astronomy, 2680 Woodlawn Drive, Honolulu, HI 96822, USA*

29 October 2019

## APPENDIX A: LINE INTENSITY RATIOS OF THE H II REGIONS

In this Appendix we include 6 tables with the line intensity ratios of the H II regions of M101 (NGC 5462, NGC 5455, H1216, NGC 5471, H37, H219, NGC 5447, H681, H1118, H1146 and SDS323) and M31 (BA289, K703, K160, BA379, BA371, BA310 and BA374) observed. Each table contains the list of line identifications and their laboratory wavelength – first 3 columns; the reddening function, $f(\lambda)$ – fourth column; the observed wavelength – fifth, seventh and ninth columns – and dereddened line intensity ratios with respect to H$\beta$ – remaining columns. Colons indicate line intensity errors of the order or greater than 40%. The last two rows of each table include the reddening coefficient and the observed –uncorrected for reddening– integrated H$\beta$ flux, $F$(H$\beta$), of the extracted aperture for each object.

This paper has been typeset from a TEX/LATEX file prepared by the author.

© 2019 The Authors

**Table A1.** Dereddened line intensity ratios with respect to $I(\mathrm{H}\beta)$ = 100 of NGC 5462, NGC 5455 and H1216 of M 101.

| $\lambda_0$ (Å) | Ion | ID | $f(\lambda)$ | NGC 5462 $\lambda$ (Å) | NGC 5462 $I(\lambda)$ | NGC 5455 $\lambda$ (Å) | NGC 5455 $I(\lambda)$ | H1216 $\lambda$ (Å) | H1216 $I(\lambda)$ |
|---|---|---|---|---|---|---|---|---|---|
| 3634.25 | He I | 28 | 0.272 | 3637.35 | 0.61 : | | – | – | – |
| 3671.48 | H I | H24 | 0.266 | – | – | 3673.42 | 0.08 : | – | – |
| 3673.76 | H I | H23 | 0.265 | – | – | 3675.69 | 0.11 : | – | – |
| 3676.37 | H I | H22 | 0.265 | – | – | 3678.44 | 0.17 : | – | – |
| 3679.36 | H I | H21 | 0.265 | – | – | 3681.36 | 0.26 : | – | – |
| 3682.81 | H I | H20 | 0.264 | – | – | 3684.80 | 0.33 : | – | – |
| 3686.83 | H I | H19 | 0.263 | 3690.22 | 0.55 : | 3688.93 | 0.51 ± 0.15 | 3690.02 | 0.48 : |
| 3691.56 | H I | H18 | 0.263 | 3695.03 | 0.61 ± 0.21 | 3693.53 | 0.65 ± 0.20 | 3695.25 | 1.47 : |
| 3697.15 | H I | H17 | 0.262 | 3700.33 | 0.78 ± 0.27 | 3699.14 | 0.81 ± 0.16 | 3700.75 | 1.28 : |
| 3703.86 | H I | H16 | 0.260 | 3707.39 | 1.17 ± 0.35 | 3706.16 | 1.21 ± 0.13 | 3707.52 | 1.81 ± 0.64 |
| 3711.97 | H I | H15 | 0.259 | 3715.35 | 1.00 ± 0.30 | 3713.98 | 1.06 ± 0.11 | 3715.40 | 1.89 ± 0.66 |
| 3721.94 | H I | H14 | 0.257 | 3725.07 | 2.29 ± 0.35 | 3723.92 | 2.57 ± 0.27 | 3725.35 | 2.66 ± 0.80 |
| 3726.03 | [O II] | 1F | 0.257 | 3729.22 | 60.2 ± 1.4 | 3728.09 | 70.7 ± 1.9 | 3729.54 | 61.6 ± 1.7 |
| 3728.82 | [O II] | 1F | 0.256 | 3732.02 | 86.8 ± 2.1 | 3730.85 | 85.9 ± 2.3 | 3732.31 | 91.6 ± 2.5 |
| 3734.37 | H I | H13 | 0.255 | 3737.50 | 1.90 ± 0.23 | 3736.32 | 1.92 ± 0.16 | 3737.87 | 2.25 ± 0.19 |
| 3750.15 | H I | H12 | 0.253 | 3753.33 | 2.16 ± 0.22 | 3752.19 | 2.21 ± 0.10 | 3753.76 | 2.43 ± 0.14 |
| 3770.63 | H I | H11 | 0.249 | 3773.86 | 2.79 ± 0.15 | 3772.69 | 2.88 ± 0.10 | 3774.21 | 3.17 ± 0.21 |
| 3784.89 | He I | 64 | 0.246 | 3788.35 | 0.16 : | – | – | – | – |
| 3797.90 | H I | H10 | 0.244 | 3801.10 | 3.43 ± 0.13 | 3799.97 | 3.87 ± 0.12 | 3801.50 | 4.20 ± 0.22 |
| 3819.61 | He I | 22 | 0.240 | 3822.82 | 0.651 ± 0.066 | 3821.70 | 0.777 ± 0.039 | 3823.47 | 0.80 ± 0.16 |
| 3835.39 | H I | H9 | 0.237 | 3838.57 | 4.93 ± 0.17 | 3837.47 | 5.57 ± 0.15 | 3839.02 | 5.61 ± 0.20 |
| 3856.02 | Si II | 1F | 0.233 | – | – | 3858.25 | 0.11 : | 3859.19 | 0.27 : |
| 3862.59 | Si II | 1 | 0.232 | – | – | 3864.66 | 0.13 : | – | – |
| 3867.49 | He I | 20 | 0.231 | 3871.97 | 21.00 ± 0.49 | 3870.87 | 20.63 ± 0.54 | 3872.39 | 25.76 ± 0.66 |
| 3868.75 | [Ne III] | 1F | 0.230 | | | | | | |
| 3888.65 | He I | | 0.226 | 3892.15 | 13.97 ± 0.33 | 3891.01 | 15.31 ± 0.39 | 3892.53 | 16.08 ± 0.44 |
| 3889.05 | H I | H8 | 0.226 | | | | | | |
| 3964.73 | He I | 5 | 0.211 | 3968.09 | 0.495 ± 0.075 | 3966.89 | 0.674 ± 0.069 | 3968.26 | 0.42 ± 0.13 |
| 3967.46 | [Ne III] | 1F | 0.211 | 3970.66 | 6.55 ± 0.16 | 3969.61 | 5.97 ± 0.15 | 3971.15 | 7.60 ± 0.20 |
| 3970.07 | H I | H7 | 0.210 | 3973.35 | 13.13 ± 0.30 | 3972.26 | 13.13 ± 0.33 | 3973.81 | 13.82 ± 0.35 |
| 4009.22 | He I | 55 | 0.202 | 4012.27 | 0.120 ± 0.042 | 4011.51 | 0.106 ± 0.016 | – | – |
| 4026.21 | He I | 18 | 0.198 | 4029.61 | 1.482 ± 0.062 | 4028.48 | 1.493 ± 0.040 | 4030.05 | 1.50 ± 0.10 |
| 4068.60 | [S II] | 1F | 0.189 | 4072.06 | 1.328 ± 0.072 | 4070.99 | 1.381 ± 0.043 | 4072.60 | 1.266 ± 0.086 |
| 4076.35 | [S II] | 1F | 0.187 | 4079.79 | 0.462 ± 0.044 | 4078.75 | 0.442 ± 0.024 | 4080.35 | 0.260 ± 0.078 |
| 4101.74 | H I | H6 | 0.182 | 4105.12 | 26.23 ± 0.57 | 4104.06 | 24.15 ± 0.57 | 4105.63 | 23.23 ± 0.56 |
| 4120.82 | He I | 16 | 0.177 | 4124.31 | 0.165 ± 0.023 | 4123.35 | 0.146 ± 0.029 | 4124.83 | 0.15 : |
| 4143.76 | He I | 53 | 0.172 | 4147.31 | 0.227 ± 0.030 | 4146.07 | 0.217 ± 0.028 | 4147.82 | 0.176 ± 0.062 |
| 4168.97 | He I | 52 | 0.167 | 4171.82 | 0.07 : | | | – | – |
| 4209.15 | [Fe III] | | 0.157 | – | – | | | – | – |
| 4243.97 | [Fe II] | 21F | 0.149 | – | – | | | – | – |
| 4267.15 | C II | 6 | 0.144 | 4270.78 | 0.124 ± 0.031 | 4269.67 | 0.107 ± 0.027 | – | – |
| 4287.40 | [Fe II] | 7F | 0.139 | 4291.13 | 0.173 ± 0.035 | 4289.89 | 0.120 ± 0.026 | 4291.92 | 0.257 ± 0.090 |
| 4340.47 | H I | Hγ | 0.127 | 4345.26 | 45.5 ± 1.0 | 4342.98 | 45.14 ± 0.99 | 4344.58 | 42.68 ± 0.95 |
| 4363.21 | [O III] | 2F | 0.121 | 4366.75 | 2.479 ± 0.079 | 4365.74 | 2.123 ± 0.080 | 4367.36 | 3.15 ± 0.13 |
| 4387.93 | He I | 51 | 0.115 | 4391.58 | 0.450 ± 0.041 | 4390.48 | 0.451 ± 0.029 | 4392.00 | 0.44 ± 0.13 |
| 4413.78 | [Fe II] | 7F | 0.109 | – | – | 4416.75 | 0.079 ± 0.028 | – | – |
| 4437.55 | He I | 50 | 0.104 | – | – | 4440.48 | 0.055 ± 0.019 | – | – |
| 4471.48 | He I | 14 | 0.096 | 4475.17 | 9.41 ± 0.23 | 4474.72 | 4.489 ± 0.099 | 4475.77 | 3.73 ± 0.11 |
| 4514.9 | [Fe II] | 6F | 0.085 | – | – | 4517.39 | 0.054 ± 0.018 | – | – |
| 4562.6 | [Mg I] | | 0.073 | – | – | | | 4566.92 | 0.405 ± 0.081 |
| 4571.1 | Mg I] | 1 | 0.071 | – | – | | | 4575.26 | 0.268 ± 0.054 |
| 4607.13 | [Fe III] | 3F | 0.062 | – | – | 4610.05 | 0.065 ± 0.017 | – | – |
| 4638.86 | O II | 1 | 0.055 | – | – | 4641.84 | 0.154 ± 0.039 | – | – |
| 4640.64 | N III | 2 | 0.054 | | | | | | |
| 4641.81 | O II | 1 | 0.054 | – | – | 4645.28 | 0.104 ± 0.021 | – | – |
| 4643.06 | N II | 5 | 0.054 | | | | | | |
| 4649.13 | O II | 1 | 0.052 | – | – | 4653.11 | 0.074 ± 0.024 | – | – |
| 4650.84 | O II | 1 | 0.052 | | | | | | |
| 4658.10 | [Fe III] | 3F | 0.050 | – | – | 4661.20 | 0.813 ± 0.044 | 4662.33 | 0.334 ± 0.034 |
| 4661.63 | O II | 1 | 0.049 | – | – | 4665.14 | 0.058 ± 0.020 | – | – |

**Table A1.** continued

| | | | | NGC 5462 | | NGC 5455 | | H1216 | |
|---|---|---|---|---|---|---|---|---|---|
| $\lambda_0$ (Å) | Ion | ID | $f(\lambda)$ | $\lambda$ (Å) | $I(\lambda)$ | $\lambda$ (Å) | $I(\lambda)$ | $\lambda$ (Å) | $I(\lambda)$ |
| 4676.24 | O II | 1 | 0.046 | – | – | – | – | 4680.70 | 0.06 : |
| 4685.71 | He II | | 0.043 | – | – | – | – | – | – |
| 4701.53 | [Fe III] | 3F | 0.039 | – | – | 4704.73 | 0.172 ± 0.027 | 4706.08 | 0.11 : |
| 4711.37 | [Ar IV] | 1F | 0.037 | – | – | 4715.99 | 0.542 ± 0.044 | – | – |
| 4713.14 | He I | 12 | 0.036 | | | | | 4717.19 | 0.635 ± 0.077 |
| 4733.93 | [Fe III] | 3F | 0.031 | – | – | 4737.19 | 0.056 ± 0.009 | – | – |
| 4740.16 | [Ar IV] | 1F | 0.030 | – | – | 4743.10 | 0.100 ± 0.022 | 4744.58 | 0.137 ± 0.041 |
| 4754.83 | [Fe III] | 3F | 0.026 | – | – | 4757.73 | 0.136 ± 0.022 | – | – |
| 4769.60 | [Fe III] | 3F | 0.023 | – | – | 4772.57 | 0.082 ± 0.016 | – | – |
| 4777.88 | [Fe III] | 3F | 0.021 | – | – | – | – | – | – |
| 4814.55 | [Fe II] | 20F | 0.012 | – | – | 4817.86 | 0.079 ± 0.030 | – | – |
| 4861.33 | H I | H$\beta$ | 0.000 | 4867.18 | 100.0 ± 3.0 | 4864.40 | 100.0 ± 2.0 | 4865.63 | 100.0 ± 2.1 |
| 4881 | [Fe III] | 2F | -0.005 | – | – | 4884.10 | 0.206 ± 0.031 | 4885.40 | 0.10 : |
| 4921.93 | He I | 48 | -0.015 | 4926.74 | 1.09 ± 0.33 | 4925.08 | 1.205 ± 0.042 | 4926.66 | 1.122 ± 0.076 |
| 4931.32 | [O III] | 1F | -0.017 | – | – | 4934.19 | 0.060 ± 0.015 | – | – |
| 4958.91 | [O III] | 1F | -0.024 | 4964.95 | 130.9 ± 2.6 | 4962.09 | 126.2 ± 2.5 | 4962.52 | 134.9 ± 2.8 |
| 4985.9 | [Fe III] | 2F | -0.031 | 4990.70 | 0.70 ± 0.25 | 4988.92 | 0.512 ± 0.040 | 4990.23 | 0.522 ± 0.053 |
| 5006.84 | [O III] | 1F | -0.036 | 5012.89 | 398.2 ± 8.6 | 5010.03 | 374.0 ± 7.5 | 5010.44 | 406.4 ± 8.2 |
| 5015.68 | He I | 4 | -0.038 | 5020.58 | 2.60 ± 0.20 | 5018.82 | 2.946 ± 0.066 | 5020.04 | 1.63 ± 0.19 |
| 5041.03 | Si II | 5 | -0.044 | – | – | 5044.25 | 0.153 ± 0.024 | 5046.01 | 0.094 ± 0.026 |
| 5047.74 | He I | 47 | -0.046 | – | – | 5050.81 | 0.164 ± 0.021 | 5052.24 | 0.153 ± 0.038 |
| 5055.98 | Si II | 5 | -0.048 | – | – | 5059.29 | 0.152 ± 0.020 | 5061.24 | 0.063 ± 0.019 |
| 5111.63 | [Fe II] | 19F | -0.061 | – | – | – | – | – | – |
| 5158.81 | [Fe II] | 19F | -0.091 | – | – | 5161.99 | 0.075 ± 0.015 | – | – |
| 5191.82 | [Ar III] | 3F | -0.081 | – | – | 5195.02 | 0.062 ± 0.013 | 5196.03 | 0.074 ± 0.027 |
| 5197.90 | [N I] | 1F | -0.082 | – | – | 5202.10 | 0.768 ± 0.040 | 5203.19 | 0.540 ± 0.034 |
| 5200.26 | [N I] | 1F | -0.083 | | | | | | |
| 5261.62 | [Fe II] | 19F | -0.109 | – | – | 5264.81 | 0.070 ± 0.014 | – | – |
| 5270.40 | [Fe III] | 1F | -0.111 | – | – | 5273.97 | 0.409 ± 0.030 | 5275.49 | 0.121 ± 0.024 |
| 5412.00 | [Fe III] | 1F | -0.136 | – | – | – | – | – | – |
| 5517.71 | [Cl III] | 1F | -0.154 | 5522.85 | 0.62 ± 0.22 | 5521.44 | 0.532 ± 0.021 | 5522.84 | 0.418 ± 0.023 |
| 5537.88 | [Cl III] | 1F | -0.158 | 5543.82 | 0.66 : | 5541.60 | 0.353 ± 0.013 | 5542.89 | 0.283 ± 0.029 |
| 5754.64 | [N II] | 3F | -0.194 | 5759.92 | 0.41 ± 0.14 | 5758.68 | 0.397 ± 0.014 | 5760.28 | 0.231 ± 0.014 |
| 5875.64 | He I | 11 | -0.215 | 5881.46 | 13.21 ± 0.38 | 5879.88 | 12.75 ± 0.32 | 5881.38 | 10.92 ± 0.28 |
| 5957.56 | Si II | 4 | -0.228 | – | – | 5962.34 | 0.086 ± 0.011 | – | – |
| 5978.93 | Si II | 4 | -0.231 | – | – | 5983.26 | 0.094 ± 0.010 | – | – |
| 6046.23 | O I | 22 | -0.242 | – | – | 6051.72 | 0.04 : | – | – |
| 6046.44 | O I | 22 | | | | | | | |
| 6046.49 | O I | 22 | | | | | | | |
| 6300.30 | [O I] | 1F | -0.282 | 6306.90 | 2.62 ± 0.20 | 6305.18 | 2.45 ± 0.11 | 6305.89 | 2.16 ± 0.14 |
| 6312.10 | [S III] | 3F | -0.283 | 6319.16 | 1.77 ± 0.22 | 6317.05 | 1.315 ± 0.083 | 6317.68 | 1.514 ± 0.079 |
| 6363.78 | [O I] | 1F | -0.291 | 6370.53 | 0.83 ± 0.12 | 6369.06 | 0.81 ± 0.12 | 6369.81 | 0.562 ± 0.094 |
| 6548.03 | [N II] | 1F | -0.318 | 6555.11 | 9.15 ± 0.51 | 6553.27 | 7.93 ± 0.25 | 6553.84 | 4.27 ± 0.15 |
| 6562.82 | H I | H$\alpha$ | -0.320 | 6570.09 | 286.2 ± 7.6 | 6567.95 | 273.0 ± 8.2 | 6568.60 | 285.1 ± 8.5 |
| 6583.41 | [N II] | 1F | -0.323 | 6590.19 | 27.67 ± 0.74 | 6588.78 | 25.65 ± 0.80 | 6589.37 | 12.89 ± 0.41 |
| 6678.15 | He I | 46 | -0.336 | 6684.84 | 3.42 ± 0.22 | 6683.65 | 3.20 ± 0.11 | 6684.30 | 3.03 ± 0.13 |
| 6716.47 | [S II] | 2F | -0.342 | 6723.34 | 17.02 ± 0.47 | 6721.93 | 15.61 ± 0.49 | 6722.79 | 12.50 ± 0.39 |
| 6730.85 | [S II] | 2F | -0.344 | 6737.74 | 13.10 ± 0.40 | 6736.38 | 12.51 ± 0.39 | 6737.20 | 9.00 ± 0.30 |
| 7002.23 | O I | 21 | -0.379 | – | – | 7008.31 | 0.07 : | – | – |
| 7065.28 | He I | 10 | -0.387 | 7075.66 | 8.11 ± 0.46 | 7074.46 | 7.09 ± 0.29 | 7075.50 | 5.33 ± 0.20 |
| 7135.78 | [Ar III] | 1F | -0.396 | 7143.05 | 10.11 ± 0.36 | 7141.83 | 7.76 ± 0.31 | 7142.48 | 6.79 ± 0.24 |
| 7236.42 | C II | 3 | -0.409 | – | – | – | – | – | – |
| 7281.35 | He I | 45 | -0.414 | – | – | 7287.13 | 0.414 ± 0.044 | 7288.12 | 0.625 ± 0.094 |
| 7318.39 | [O II] | 2F | -0.418 | 7327.32 | 1.80 ± 0.29 | 7326.02 | 1.93 ± 0.17 | 7326.67 | 1.85 ± 0.11 |
| 7319.99 | [O II] | 2F | -0.418 | | | | | | |
| 7329.66 | [O II] | 2F | -0.420 | 7337.19 | 1.13 ± 0.20 | 7336.50 | 1.59 ± 0.17 | 7336.96 | 1.59 ± 0.10 |
| 7330.73 | [O II] | 2F | -0.420 | | | | | | |
| 7751.10 | [Ar III] | 2F | -0.467 | 7758.70 | 2.32 ± 0.24 | 7757.45 | 1.52 ± 0.10 | 7758.27 | 1.54 ± 0.12 |
| $c$(H$\beta$) | | | | 0.03 ± 0.02 | | 0.06 ± 0.03 | | 0.34 ± 0.03 | |
| $F$(H$\beta$) ($10^{-14}$ erg cm$^{-2}$ s$^{-1}$) | | | | 2.54 ± 008 | | 7.57± 0.15 | | 5.48 ± 0.11 | |

**Table A2.** Dereddened line intensity ratios with respect to $I(\mathrm{H}\beta)$ = 100 of NGC 5471, H37 and H219 of M 101.

| | | | | NGC 5471 | | H37 | | H219 | |
|---|---|---|---|---|---|---|---|---|---|
| $\lambda_0$ (Å) | Ion | ID | $f(\lambda)$ | $\lambda$ (Å) | $I(\lambda)$ | $\lambda$ (Å) | $I(\lambda)$ | $\lambda$ (Å) | $I(\lambda)$ |
| 3686.83 | H I | H19 | 0.263 | 3690.315 | 0.77 ± 0.11 | – | – | – | – |
| 3691.56 | H I | H18 | 0.263 | 3694.998 | 0.91 ± 0.11 | – | – | – | – |
| 3697.15 | H I | H17 | 0.262 | 3700.61 | 1.014 ± 0.095 | – | – | – | – |
| 3703.86 | H I | H16 | 0.260 | 3707.654 | 1.55 ± 0.13 | 3706.86 | 2.09 ± 0.63 | – | – |
| 3711.97 | H I | H15 | 0.259 | 3715.462 | 1.25 ± 0.10 | – | – | – | – |
| 3721.94 | H I | H14 | 0.257 | 3725.478 | 2.83 ± 0.14 | 3724.88 | 3.45 ± 0.86 | – | – |
| 3726.03 | [O II] | 1F | 0.257 | 3729.531 | 38.0 ± 1.0 | 3728.97 | 91.0 ± 2.4 | 3728.17 | 113.7 ± 3.1 |
| 3728.82 | [O II] | 1F | 0.256 | 3732.28 | 48.0 ± 1.3 | 3731.74 | 136.3 ± 3.7 | 3730.94 | 173.1 ± 4.7 |
| 3734.37 | H I | H13 | 0.255 | 3737.854 | 2.10 ± 0.10 | 3737.23 | 3.46 ± 0.53 | 3736.38 | 1.59 ± 0.56 |
| 3750.15 | H I | H12 | 0.253 | 3753.712 | 2.335 ± 0.074 | 3753.28 | 3.41 ± 0.30 | 3752.35 | 2.09 ± 0.44 |
| 3770.63 | H I | H11 | 0.249 | 3774.222 | 3.086 ± 0.091 | 3773.68 | 3.72 ± 0.34 | 3772.94 | 3.28 ± 0.43 |
| 3784.89 | He I | 64 | 0.246 | 3788.613 | 0.08 : | – | – | – | – |
| 3797.90 | H I | H10 | 0.244 | 3801.503 | 4.18 ± 0.12 | 3800.91 | 5.66 ± 0.51 | 3800.09 | 3.67 ± 0.42 |
| 3819.61 | He I | 22 | 0.240 | 3823.282 | 0.743 ± 0.042 | 3822.67 | 1.14 ± 0.40 | 3821.83 | 0.97 ± 0.38 |
| 3835.39 | H I | H9 | 0.237 | 3839.039 | 5.92 ± 0.16 | 3838.44 | 6.57 ± 0.31 | 3837.64 | 5.75 ± 0.38 |
| 3856.02 | Si II | 1F | 0.233 | | – | 3860.26 | 0.33 ± 0.12 | – | – |
| 3867.49 | He I | 20 | 0.231 | 3872.443 | 48.9 ± 1.3 | 3871.85 | 29.47 ± 0.88 | 3870.96 | 5.41 ± 0.33 |
| 3868.75 | [Ne III] | 1F | 0.230 | | | | | | |
| 3888.65 | He I | | 0.226 | 3892.567 | 17.42 ± 0.45 | 3891.98 | 20.31 ± 0.63 | 3891.13 | 15.71 ± 0.50 |
| 3889.05 | H I | H8 | 0.226 | | | | | | |
| 3964.73 | He I | 5 | 0.211 | 3968.544 | 0.563 ± 0.031 | 3966.88 | 0.80 ± 0.28 | – | – |
| 3967.46 | [Ne III] | 1F | 0.211 | 3971.217 | 16.56 ± 0.44 | 3970.59 | 10.23 ± 0.33 | 3969.64 | 1.46 ± 0.29 |
| 3970.07 | H I | H7 | 0.210 | 3973.842 | 15.38 ± 0.41 | 3973.22 | 17.45 ± 0.56 | 3972.41 | 13.62 ± 0.43 |
| 4009.22 | He I | 55 | 0.202 | 4012.977 | 0.149 ± 0.019 | – | – | – | – |
| 4026.21 | He I | 18 | 0.198 | 4030.021 | 1.613 ± 0.048 | 4029.42 | 1.94 ± 0.15 | 4028.69 | 1.25 ± 0.16 |
| 4068.60 | [S II] | 1F | 0.189 | 4072.52 | 1.215 ± 0.048 | 4071.98 | 1.28 ± 0.13 | 4070.97 | 1.406 ± 0.091 |
| 4076.35 | [S II] | 1F | 0.187 | 4080.194 | 0.353 ± 0.034 | 4079.52 | 0.41 ± 0.10 | 4078.88 | 0.36 ± 0.13 |
| 4101.74 | H I | H6 | 0.182 | 4105.581 | 24.79 ± 0.59 | 4105.00 | 25.60 ± 0.63 | 4104.19 | 22.72 ± 0.62 |
| 4120.82 | He I | 16 | 0.177 | 4124.679 | 0.163 ± 0.020 | – | – | – | – |
| 4143.76 | He I | 53 | 0.172 | 4147.678 | 0.221 ± 0.022 | – | – | – | – |
| 4243.97 | [Fe II] | 21F | 0.149 | 4248.052 | 0.072 ± 0.022 | – | – | – | – |
| 4267.15 | C II | 6 | 0.144 | 4271.347 | 0.054 ± 0.016 | 4270.73 | 0.099 ± 0.035 | 4269.54 | – |
| 4287.40 | [Fe II] | 7F | 0.139 | 4291.535 | 0.089 ± 0.024 | – | – | – | – |
| 4340.47 | H I | H$\gamma$ | 0.127 | 4344.432 | 47.7 ± 1.0 | 4343.89 | 46.8 ± 1.8 | 4343.09 | 44.6 ± 1.1 |
| 4363.21 | [O III] | 2F | 0.121 | 4367.194 | 10.55 ± 0.24 | 4366.70 | 3.28 ± 0.18 | 4365.80 | 1.15 ± 0.21 |
| 4387.93 | He I | 51 | 0.115 | 4391.963 | 0.395 ± 0.015 | 4391.56 | 0.431 ± 0.065 | – | – |
| 4413.78 | [Fe II] | 7F | 0.109 | 4418.878 | 0.117 ± 0.033 | – | – | – | – |
| 4437.55 | He I | 50 | 0.104 | 4441.796 | 0.053 ± 0.017 | – | – | – | – |
| 4471.48 | He I | 14 | 0.096 | 4475.883 | 3.786 ± 0.084 | 4474.60 | 3.77 ± 0.21 | 4474.80 | 3.33 ± 0.20 |
| 4562.6 | [Mg I] | | 0.073 | 4567.02 | 0.232 ± 0.033 | – | – | – | – |
| 4571.1 | Mg I] | 1 | 0.071 | 4575.505 | 0.197 ± 0.028 | 4574.35 | 0.49 ± 0.15 | – | – |
| 4607.13 | [Fe III] | 3F | 0.062 | 4611.728 | 0.057 ± 0.020 | – | – | – | – |
| 4638.86 | O II | 1 | 0.055 | 4645.215 | 0.064 ± 0.022 | – | – | – | – |
| 4640.64 | N III | 2 | 0.054 | | | | | | |
| 4649.13 | O II | 1 | 0.052 | 4654.921 | 0.050 ± 0.017 | – | – | – | – |
| 4650.84 | O II | 1 | 0.052 | | | | | | |
| 4658.10 | [Fe III] | 3F | 0.050 | 4662.987 | 0.720 ± 0.029 | – | – | – | – |
| 4685.71 | He II | | 0.043 | 4690.25 | 0.632 ± 0.029 | – | – | – | – |
| 4701.53 | [Fe III] | 3F | 0.039 | 4706.334 | 0.160 ± 0.022 | – | – | – | – |
| 4711.37 | [Ar IV] | 1F | 0.037 | 4716.434 | 1.659 ± 0.044 | – | – | – | – |
| 4713.14 | He I | 12 | 0.036 | | | 4716.76 | 0.58 ± 0.20 | – | – |
| 4733.93 | [Fe III] | 3F | 0.031 | 4738.724 | 0.038 ± 0.011 | – | – | – | – |
| 4740.16 | [Ar IV] | 1F | 0.030 | 4744.87 | 0.887 ± 0.023 | – | – | – | – |
| 4754.83 | [Fe III] | 3F | 0.026 | 4759.404 | 0.136 ± 0.017 | – | – | – | – |
| 4769.60 | [Fe III] | 3F | 0.023 | 4774.464 | 0.044 ± 0.013 | – | – | – | – |
| 4777.88 | [Fe III] | 3F | 0.021 | 4782.091 | 0.023 ± 0.008 | – | – | – | – |
| 4814.55 | [Fe II] | 20F | 0.012 | 4819.565 | 0.035 ± 0.010 | – | – | – | – |
| 4861.33 | H I | H$\beta$ | 0.000 | 4865.99 | 100.0 ± 2.0 | 4864.87 | 100.0 ± 2.0 | 4864.55 | 100.0 ± 2.0 |
| 4881 | [Fe III] | 2F | -0.005 | 4885.713 | 0.189 ± 0.019 | – | – | – | – |
| 4921.93 | He I | 48 | -0.015 | 4926.609 | 0.948 ± 0.035 | 4925.40 | 0.83 ± 0.18 | 4925.53 | 0.88 ± 0.10 |

**Table A2.** continued

| | | | | NGC 5471 | | H37 | | H219 | |
|---|---|---|---|---|---|---|---|---|---|
| $\lambda_0$ (Å) | Ion | ID | $f(\lambda)$ | $\lambda$ (Å) | $I(\lambda)$ | $\lambda$ (Å) | $I(\lambda)$ | $\lambda$ (Å) | $I(\lambda)$ |
| 4931.32 | [O III] | 1F | -0.017 | 4935.852 | 0.090 ± 0.016 | – | – | – | – |
| 4958.91 | [O III] | 1F | -0.024 | 4963.657 | 217.9 ± 4.4 | 4962.64 | 126.4 ± 2.6 | 4962.13 | 63.6 ± 1.3 |
| 4985.9 | [Fe III] | 2F | -0.031 | | – | – | – | 4989.60 | 0.80 ± 0.17 |
| 5006.84 | [O III] | 1F | -0.036 | 5011.63 | 649.6 ± 13.1 | 5010.60 | 376.5 ± 7.6 | 5010.08 | 190.8 ± 3.9 |
| 5015.68 | He I | 4 | -0.038 | 5020.538 | 2.302 ± 0.083 | – | – | 5018.98 | 2.26 ± 0.16 |
| 5041.03 | Si II | 5 | -0.044 | 5045.908 | 0.075 ± 0.010 | – | – | – | – |
| 5047.74 | He I | 47 | -0.046 | 5052.5 | 0.133 ± 0.014 | – | – | – | – |
| 5055.98 | Si II | 5 | -0.048 | 5060.824 | 0.040 ± 0.010 | – | – | – | – |
| 5111.63 | [Fe II] | 19F | -0.061 | 5117.037 | 0.0198 ± 0.0050 | – | – | – | – |
| 5158.81 | [Fe II] | 19F | -0.091 | 5164.214 | 0.111 ± 0.015 | – | – | – | – |
| 5191.82 | [Ar III] | 3F | -0.081 | 5196.395 | 0.086 ± 0.014 | – | – | – | – |
| 5197.90 | [N I] | 1F | -0.082 | 5203.498 | 0.318 ± 0.019 | 5202.21 | 0.780 ± 0.089 | 5202.53 | 0.65 ± 0.13 |
| 5200.26 | [N I] | 1F | -0.083 | | | | | | |
| 5261.62 | [Fe II] | 19F | -0.109 | 5266.755 | 0.052 ± 0.013 | – | – | – | – |
| 5270.40 | [Fe III] | 1F | -0.111 | 5275.701 | 0.285 ± 0.024 | – | – | – | – |
| 5412.00 | [Fe III] | 1F | -0.136 | 5416.753 | 0.037 ± 0.009 | – | – | – | – |
| 5517.71 | [Cl III] | 1F | -0.154 | 5522.922 | 0.352 ± 0.019 | 5521.73 | 0.380 ± 0.070 | 5521.32 | 0.558 ± 0.093 |
| 5537.88 | [Cl III] | 1F | -0.158 | 5543.08 | 0.240 ± 0.015 | 5542.99 | 0.257 ± 0.077 | 5541.56 | 0.46 ± 0.10 |
| 5754.64 | [N II] | 3F | -0.194 | 5760.147 | 0.128 ± 0.010 | 5759.00 | 0.261 ± 0.092 | 5758.67 | 0.541 ± 0.077 |
| 5875.64 | He I | 11 | -0.215 | 5881.387 | 9.69 ± 0.24 | 5880.17 | 9.40 ± 0.28 | 5879.87 | 11.17 ± 0.33 |
| 5957.56 | Si II | 4 | -0.228 | 5963.823 | 0.0381 ± 0.0045 | – | – | – | – |
| 5978.93 | Si II | 4 | -0.231 | 5984.799 | 0.0510 ± 0.0052 | – | – | – | – |
| 6046.23 | O I | 22 | -0.242 | 6051.566 | 0.024 ± 0.011 | – | – | – | – |
| 6046.44 | O I | 22 | | | | | | | |
| 6046.49 | O I | 22 | | | | | | | |
| 6300.30 | [O I] | 1F | -0.282 | 6305.716 | 2.133 ± 0.087 | 6305.05 | 2.21 ± 0.13 | – | – |
| 6312.10 | [S III] | 3F | -0.283 | 6317.583 | 1.424 ± 0.058 | 6317.07 | 1.291 ± 0.097 | 6317.66 | 1.17 ± 0.20 |
| 6363.78 | [O I] | 1F | -0.291 | 6369.308 | 0.750 ± 0.048 | 6368.53 | 0.780 ± 0.081 | – | – |
| 6548.03 | [N II] | 1F | -0.318 | 6552.863 | 1.213 ± 0.051 | 6553.15 | 4.54 ± 0.19 | 6553.26 | 10.25 ± 0.43 |
| 6562.82 | H I | H$\alpha$ | -0.320 | 6568.3 | 281.2 ± 7.1 | 6568.00 | 283.5 ± 6.8 | 6568.44 | 277.8 ± 8.3 |
| 6583.41 | [N II] | 1F | -0.323 | 6589.16 | 5.42 ± 0.20 | 6588.56 | 13.18 ± 0.48 | 6589.12 | 35.1 ± 1.1 |
| 6678.15 | He I | 46 | -0.336 | 6684.073 | 2.511 ± 0.081 | 6683.45 | 2.52 ± 0.11 | 6683.71 | 2.97 ± 0.27 |
| 6716.47 | [S II] | 2F | -0.342 | 6722.354 | 7.08 ± 0.22 | 6721.68 | 12.23 ± 0.45 | 6722.39 | 23.15 ± 0.75 |
| 6730.85 | [S II] | 2F | -0.344 | 6736.848 | 5.69 ± 0.18 | 6736.06 | 8.62 ± 0.32 | 6736.78 | 16.24 ± 0.53 |
| 7065.28 | He I | 10 | -0.387 | 7073.88 | 4.91 ± 0.19 | 7075.16 | 6.32 ± 0.29 | 7075.95 | 10.24 ± 0.47 |
| 7135.78 | [Ar III] | 1F | -0.396 | 7142.177 | 5.02 ± 0.18 | 7141.51 | 5.47 ± 0.22 | 7142.31 | 6.93 ± 0.32 |
| 7236.42 | C II | 3 | -0.409 | 7243.821 | 0.089 ± 0.027 | – | – | – | – |
| 7281.35 | He I | 45 | -0.414 | 7287.641 | 0.394 ± 0.049 | 7286.75 | 0.48 ± 0.12 | 7286.86 | 0.353 ± 0.089 |
| 7318.39 | [O II] | 2F | -0.418 | 7326.685 | 1.34 ± 0.10 | 7325.47 | 1.75 ± 0.19 | 7325.50 | 2.51 ± 0.39 |
| 7319.99 | [O II] | 2F | -0.418 | | | | | | |
| 7329.66 | [O II] | 2F | -0.420 | 7337.335 | 1.055 ± 0.083 | 7336.31 | 1.55 ± 0.16 | 7335.75 | 2.74 ± 0.42 |
| 7330.73 | [O II] | 2F | -0.420 | | | | | | |
| 7751.10 | [Ar III] | 2F | -0.467 | 7757.971 | 1.13 ± 0.12 | 7757.30 | 0.869 ± 0.093 | 7757.27 | 1.13 ± 0.25 |
| $c$(H$\beta$) | | | | 0.00 ± 0.03 | | 0.21 ± 0.03 | | 0.09 ± 0.03 | |
| $F$(H$\beta$) ($10^{-14}$ erg cm$^{-2}$ s$^{-1}$) | | | | 10.90 ± 0.22 | | 5.48 ± 0.11 | | 7.23 ± 0.14 | |

**Table A3.** Dereddened line intensity ratios with respect to $I(\mathrm{H}\beta)$ = 100 of NGC 5447, H681, and H1118 of M 101.

| | | | | NGC 5447 | | H681 | | H1118 | |
|---|---|---|---|---|---|---|---|---|---|
| $\lambda_0$ (Å) | Ion | ID | $f(\lambda)$ | $\lambda$ (Å) | $I(\lambda)$ | $\lambda$ (Å) | $I(\lambda)$ | $\lambda$ (Å) | $I(\lambda)$ |
| 3686.83 | H I | H19 | 3688.92 | 0.69 ± 0.11 | – | – | | | |
| 3691.56 | H I | H18 | 3693.77 | 0.84 ± 0.14 | – | – | | | |
| 3697.15 | H I | H17 | 3699.23 | 1.05 ± 0.12 | – | – | – | – | |
| 3703.86 | H I | H16 | 3706.22 | 1.50 ± 0.17 | – | – | – | – | |
| 3711.97 | H I | H15 | 3714.03 | 1.26 ± 0.10 | – | – | – | – | |
| 3721.94 | H I | H14 | 3724.20 | 3.01 ± 0.17 | – | – | – | – | |
| 3726.03 | [O II] | 1F | 3728.10 | 51.5 ± 1.4 | 3729.28 | 71.9 ± 1.7 | 3729.78 | 97.3 ± 2.6 | |
| 3728.82 | [O II] | 1F | 3730.88 | 67.9 ± 1.8 | 3732.06 | 106.9 ± 2.5 | 3732.56 | 143.3 ± 3.9 | |
| 3734.37 | H I | H13 | 3736.34 | 2.23 ± 0.13 | | – | – | – | |
| 3750.15 | H I | H12 | 3752.19 | 2.31 ± 0.14 | 3753.69 | 2.03 ± 0.61 | 3754.22 | 4.8 ± 1.7 | |
| 3770.63 | H I | H11 | 3772.70 | 3.08 ± 0.13 | 3773.82 | 3.42 ± 0.56 | 3774.07 | 4.3 ± 1.5 | |
| 3797.90 | H I | H10 | 3800.00 | 4.26 ± 0.15 | 3801.23 | 4.28 ± 0.58 | 3801.78 | 4.1 ± 1.2 | |
| 3819.61 | He I | 22 | 3821.72 | 0.85 ± 0.12 | – | – | – | – | |
| 3835.39 | H I | H9 | 3837.51 | 6.16 ± 0.17 | 3838.71 | 5.58 ± 0.57 | 3839.22 | 3.1 ± 1.1 | |
| 3867.49 | He I | 20 | 3870.92 | 23.95 ± 0.62 | 3872.19 | 24.67 ± 0.74 | 3872.62 | 31.7 ± 1.3 | |
| 3868.75 | [Ne III] | 1F | | | | | | | |
| 3888.65 | He I | | 3891.04 | 17.72 ± 0.46 | 3892.28 | 17.28 ± 0.55 | 3892.75 | 19.02 ± 0.91 | |
| 3889.05 | H I | H8 | | | | | | | |
| 3964.73 | He I | 5 | 3967.11 | 0.557 ± 0.085 | – | – | – | – | |
| 3967.46 | [Ne III] | 1F | 3969.67 | 6.68 ± 0.21 | 3970.95 | 7.52 ± 0.63 | 3971.35 | 7.33 ± 0.90 | |
| 3970.07 | H I | H7 | 3972.31 | 14.38 ± 0.38 | 3973.60 | 14.26 ± 0.65 | 3974.02 | 14.9 ± 1.1 | |
| 4009.22 | He I | 55 | 4011.57 | 0.110 ± 0.022 | – | – | – | – | |
| 4026.21 | He I | 18 | 4028.57 | 1.603 ± 0.053 | 4029.69 | 1.45 ± 0.29 | 4030.73 | 2.06 ± 0.72 | |
| 4068.60 | [S II] | 1F | 4071.11 | 0.875 ± 0.051 | 4072.36 | 1.64 ± 0.33 | 4072.61 | 1.78 ± 0.62 | |
| 4076.35 | [S II] | 1F | 4078.75 | 0.233 ± 0.023 | 4079.68 | 0.33 : | – | – | |
| 4101.74 | H I | H6 | 4104.14 | 24.04 ± 0.57 | 4105.42 | 25.84 ± 0.63 | 4105.86 | 24.71 ± 0.84 | |
| 4120.82 | He I | 16 | 4123.09 | 0.090 ± 0.027 | – | – | – | – | |
| 4143.76 | He I | 53 | 4146.23 | 0.207 ± 0.025 | – | – | – | – | |
| 4267.15 | C II | 6 | 4269.66 | 0.103 ± 0.026 | – | – | – | – | |
| 4287.40 | [Fe II] | 7F | 4289.93 | 0.115 ± 0.026 | – | – | – | – | |
| 4340.47 | H I | H$\gamma$ | 4343.09 | 46.3 ± 1.0 | 4344.42 | 47.0 ± 1.4 | 4344.86 | 47.3 ± 1.5 | |
| 4363.21 | [O III] | 2F | 4365.88 | 1.993 ± 0.067 | 4367.24 | 4.81 ± 0.29 | 4367.80 | 5.99 ± 0.66 | |
| 4387.93 | He I | 51 | 4390.64 | 0.428 ± 0.037 | – | – | – | – | |
| 4471.48 | He I | 14 | 4474.24 | 3.904 ± 0.088 | 4475.64 | 3.13 ± 0.16 | 4477.77 | 4.00 : | |
| 4562.6 | [Mg I] | | 4565.27 | 0.104 ± 0.031 | – | – | – | – | |
| 4571.1 | Mg I] | 1 | 4574.05 | 0.115 ± 0.040 | – | – | – | – | |
| 4685.71 | He II | | – | – | 4690.14 | 0.28 : | – | – | |
| 4711.37 | [Ar IV] | 1F | – | – | 4716.67 | 0.44 ± 0.13 | – | – | |
| 4713.14 | He I | 12 | | – | | | – | – | |
| 4861.33 | H I | H$\beta$ | 4864.33 | 100.0 ± 2.1 | 4865.62 | 100.0 ± 2.0 | 4866.05 | 100.0 ± 2.1 | |
| 4921.93 | He I | 48 | 4924.59 | 1.22 ± 0.43 | 4926.35 | 0.58 ± 0.09 | – | – | |
| 4958.91 | [O III] | 1F | 4962.08 | 131.3 ± 2.7 | 4963.21 | 102.8 ± 2.1 | 4963.72 | 158.7 ± 3.4 | |
| 4985.9 | [Fe III] | 2F | – | – | – | – | – | – | |
| 5006.84 | [O III] | 1F | 5010.07 | 394.2 ± 8.0 | 5011.16 | 305.7 ± 6.1 | 5011.64 | 473.9 ± 9.7 | |
| 5015.68 | He I | 4 | 5021.44 | 23.7 ± 1.3 | 5020.15 | 1.89 ± 0.15 | – | – | |
| 5197.90 | [N I] | 1F | – | – | – | – | – | – | |
| 5200.26 | [N I] | 1F | | | | | | | |
| 5517.71 | [Cl III] | 1F | – | – | 5522.39 | 0.25 : | – | – | |
| 5537.88 | [Cl III] | 1F | – | – | 5542.94 | 0.26 : | – | – | |
| 5754.64 | [N II] | 3F | – | – | 5759.33 | 0.15 : | – | – | |
| 5875.64 | He I | 11 | 5880.51 | 13.8 ± 1.3 | 5881.31 | 9.16 ± 0.26 | 5881.57 | 9.64 ± 0.76 | |
| 6300.30 | [O I] | 1F | 6303.85 | 1.26 ± 0.38 | – | – | – | – | |
| 6312.10 | [S III] | 3F | 6316.49 | 1.25 ± 0.38 | 6318.99 | 1.07 ± 0.27 | 6317.85 | 2.90 ± 0.87 | |
| 6548.03 | [N II] | 1F | 6552.35 | 5.48 ± 0.32 | 6553.96 | 3.48 ± 0.53 | 6554.86 | 5.16 ± 0.79 | |
| 6562.82 | H I | H$\alpha$ | 6567.16 | 287.6 ± 8.6 | 6568.85 | 280.8 ± 7.0 | 6569.82 | 281.6 ± 8.5 | |
| 6583.41 | [N II] | 1F | 6587.63 | 16.74 ± 0.60 | 6589.58 | 10.34 ± 0.49 | 6590.72 | 18.0 ± 1.0 | |
| 6678.15 | He I | 46 | 6682.36 | 2.75 ± 0.20 | 6684.34 | 2.56 ± 0.20 | 6685.29 | 2.65 ± 0.29 | |
| 6716.47 | [S II] | 2F | 6720.61 | 10.18 ± 0.44 | 6722.84 | 16.27 ± 0.64 | 6723.88 | 20.84 ± 0.88 | |
| 6730.85 | [S II] | 2F | 6735.16 | 7.69 ± 0.33 | 6737.22 | 11.78 ± 0.46 | 6738.35 | 14.68 ± 0.84 | |
| 7065.28 | He I | 10 | 7072.83 | 5.70 ± 0.74 | 7076.36 | 7.61 ± 0.62 | 7078.73 | 13.0 ± 1.5 | |

**Table A3.** continued

| $\lambda_0$ (Å) | Ion | ID | $f(\lambda)$ | NGC 5447 $\lambda$ (Å) | NGC 5447 $I(\lambda)$ | H681 $\lambda$ (Å) | H681 $I(\lambda)$ | H1118 $\lambda$ (Å) | H1118 $I(\lambda)$ |
|---|---|---|---|---|---|---|---|---|---|
| 7135.78 | [Ar III] | 1F | 7140.72 | 7.48 ± 0.61 | 7142.63 | 4.19 ± 0.42 | 7143.64 | 8.61 ± 0.74 | |
| $c(\mathrm{H}\beta)$ | | | | 0.00 ± 0.03 | | 0.13 ± 0.08 | | 0.05 ± 0.03 | |
| $F(\mathrm{H}\beta)$ ($10^{-14}$ erg cm$^{-2}$ s$^{-1}$) | | | | 6.01 ± 0.12 | | 0.87 ± 0.02 | | 2.98 ± 0.06 | |

**Table A4.** Dereddened line intensity ratios with respect to $I(\mathrm{H}\beta)$ = 100 of H1146 and SDH323 of M 101 and BA289 of M 31.

| $\lambda_0$ (Å) | Ion | ID | $f(\lambda)$ | H1146 $\lambda$ (Å) | H1146 $I(\lambda)$ | SDH323 $\lambda$ (Å) | SDH323 $I(\lambda)$ | BA289 $\lambda$ (Å) | BA289 $I(\lambda)$ |
|---|---|---|---|---|---|---|---|---|---|
| 3726.03 | [O II] | 1F | 0.257 | 3729.82 | 74.0 ± 2.5 | 3728.40 | 47.1 ± 2.6 | 3719.70 | 46.1 ± 1.3 |
| 3728.82 | [O II] | 1F | 0.256 | 3732.50 | 105.4 ± 3.5 | 3731.27 | 106.7 ± 5.8 | 3722.49 | 82.5 ± 2.4 |
| 3770.63 | H I | H11 | 0.249 | – | – | 3773.48 | 2.50 ± 0.88 | – | – |
| 3797.90 | H I | H10 | 0.244 | 3801.57 | 5.4 ± 1.7 | 3800.75 | 4.46 ± 0.70 | 3791.41 | 3.50 ± 0.74 |
| 3835.39 | H I | H9 | 0.237 | 3838.95 | 6.2 : | 3838.17 | 4.47 ± 0.92 | 3828.86 | 5.5 ± 1.1 |
| 3867.49 | He I | 20 | 0.231 | 3872.67 | 38.0 ± 2.8 | 3871.65 | 17.5 ± 1.6 | – | – |
| 3868.75 | [Ne III] | 1F | 0.230 | | | | | | |
| 3888.65 | He I | | 0.226 | 3892.81 | 20.0 ± 2.4 | 3891.73 | 17.1 ± 1.5 | 3882.36 | 15.3 ± 1.5 |
| 3889.05 | H I | H8 | 0.226 | | | | | | |
| 3967.46 | [Ne III] | 1F | 0.211 | 3971.36 | 14.1 ± 2.1 | 3970.39 | 3.76 ± 0.58 | – | – |
| 3970.07 | H I | H7 | 0.210 | 3974.07 | 13.3 ± 1.6 | 3973.04 | 14.9 ± 1.6 | 3963.34 | 11.63 ± 0.89 |
| 4026.21 | He I | 18 | 0.198 | – | – | 4028.87 | 1.43 ± 0.50 | – | – |
| 4068.60 | [S II] | 1F | 0.189 | – | – | 4071.78 | 0.88 : | – | – |
| 4101.74 | H I | H6 | 0.182 | 4105.85 | 25.0 ± 1.3 | 4104.97 | 22.6 ± 1.4 | 4094.74 | 24.09 ± 0.82 |
| 4340.47 | H I | Hγ | 0.127 | 4344.79 | 48.1 ± 1.5 | 4344.08 | 43.9 ± 1.8 | 4332.99 | 43.7 ± 1.2 |
| 4363.21 | [O III] | 2F | 0.121 | 4367.70 | 4.7 ± 1.2 | 4366.85 | 4.03 ± 0.44 | 4358.84 | 0.49 ± 0.16 |
| 4471.48 | He I | 14 | 0.096 | 4476.10 | 4.03 ± 0.88 | 4475.36 | 3.55 ± 0.37 | 4464.03 | 2.74 ± 0.23 |
| 4711.37 | [Ar IV] | 1F | 0.037 | 4708.26 | 2.19 ± 0.69 | – | – | – | – |
| 4713.14 | He I | 12 | 0.036 | | | | | | |
| 4861.33 | H I | Hβ | 0.000 | 4866.14 | 100.0 ± 2.6 | 4866.41 | 100.0 ± 2.3 | 4853.21 | 100.0 ± 2.0 |
| 4921.93 | He I | 48 | -0.015 | – | – | – | ± | 4914.02 | 0.68 ± 0.11 |
| 4958.91 | [O III] | 1F | -0.024 | 4963.92 | 150.3 ± 3.3 | 4964.10 | 73.1 ± 1.9 | 4950.61 | 7.91 ± 0.24 |
| 4985.9 | [Fe III] | 2F | -0.031 | – | – | – | ± | 4977.95 | 0.60 ± 0.14 |
| 5006.84 | [O III] | 1F | -0.036 | 5011.90 | 447.4 ± 9.4 | 5012.08 | 213.2 ± 4.7 | 4998.47 | 23.72 ± 0.67 |
| 5015.68 | He I | 4 | -0.038 | – | – | – | – | 5007.27 | 1.48 ± 0.19 |
| 5197.90 | [N I] | 1F | -0.082 | – | – | – | – | 5190.30 | 1.52 ± 0.23 |
| 5200.26 | [N I] | 1F | -0.083 | | | | | | |
| 5754.64 | [N II] | 3F | -0.194 | – | – | – | – | 5745.53 | 0.48 ± 0.11 |
| 5875.64 | He I | 11 | -0.215 | 5881.77 | 9.66 ± 0.84 | 5881.97 | 8.8 ± 1.4 | 5865.91 | 9.76 ± 0.33 |
| 6312.10 | [S III] | 3F | -0.283 | 6319.03 | 2.34 ± 0.87 | – | – | – | – |
| 6548.03 | [N II] | 1F | -0.318 | 6554.46 | 7.77 ± 0.81 | – | – | 6536.66 | 34.56 ± 1.46 |
| 6562.82 | H I | Hα | -0.320 | 6569.72 | 283.3 ± 8.9 | 6569.65 | 273 ± 15 | 6551.34 | 280.3 ± 8.4 |
| 6583.41 | [N II] | 1F | -0.323 | 6590.37 | 19.9 ± 1.5 | 6590.04 | 8.4 ± 1.2 | 6571.97 | 101.3 ± 3.1 |
| 6678.15 | He I | 46 | -0.336 | 6685.71 | 3.19 ± 0.96 | 6686.13 | 4.1 ± 1.3 | 6666.38 | 2.43 ± 0.32 |
| 6716.47 | [S II] | 2F | -0.342 | 6723.46 | 18.21 ± 0.88 | 6723.26 | 10.6 ± 1.0 | 6704.77 | 34.5 ± 1.4 |
| 6730.85 | [S II] | 2F | -0.344 | 6737.68 | 12.95 ± 0.70 | 6738.39 | 8.21 ± 0.84 | 6719.14 | 24.6 ± 1.1 |
| 7065.28 | He I | 10 | -0.387 | 7078.18 | 6.1 ± 1.5 | 7076.72 | 7.4 ± 2.3 | 7055.04 | 4.14 ± 0.46 |
| 7135.78 | [Ar III] | 1F | -0.396 | 7143.32 | 8.17 ± 0.82 | 7143.73 | 2.42 ± 0.74 | 7123.53 | 2.84 ± 0.21 |
| $c(\mathrm{H}\beta)$ | | | | 0.14 ± 0.03 | | 0.00 ± 0.07 | | 0.36 ± 0.03 | |
| $F(\mathrm{H}\beta)$ ($10^{-14}$ erg cm$^{-2}$ s$^{-1}$) | | | | 4.34 ± 0.09 | | 0.343 ± 0.007 | | 0.59 ± 0.01 | |

**Table A5.** Dereddened line intensity ratios with respect to $I(\mathrm{H}\beta)$ = 100 of K703, K160 and BA379 of M 31.

| | | | | K703 | | K160 | | BA379 | |
|---|---|---|---|---|---|---|---|---|---|
| $\lambda_0$ (Å) | Ion | ID | $f(\lambda)$ | $\lambda$ (Å) | $I(\lambda)$ | $\lambda$ (Å) | $I(\lambda)$ | $\lambda$ (Å) | $I(\lambda)$ |
| 3721.94 | H I | H14 | 0.257 | – | – | – | – | 3714.23 | 2.18 ± 0.33 |
| 3726.03 | [O II] | 1F | 0.257 | 3723.72 | 68.7 ± 1.8 | 3722.04 | 101.0 ± 2.8 | 3718.41 | 73.4 ± 1.7 |
| 3728.82 | [O II] | 1F | 0.256 | 3726.50 | 103.9 ± 2.8 | 3724.81 | 140.1 ± 3.9 | 3721.16 | 109.2 ± 2.5 |
| 3734.37 | H I | H13 | 0.255 | – | – | – | – | 3726.92 | 3.24 ± 0.52 |
| 3750.15 | H I | H12 | 0.253 | – | – | 3745.75 | 2.42 ± 0.59 | 3742.32 | 3.10 ± 0.33 |
| 3770.63 | H I | H11 | 0.249 | 3767.94 | 2.79 ± 0.98 | 3766.58 | 3.66 ± 0.64 | 3763.00 | 4.02 ± 0.61 |
| 3797.90 | H I | H10 | 0.244 | 3795.47 | 2.83 ± 0.71 | 3793.91 | 5.59 ± 0.56 | 3790.14 | 4.90 ± 0.28 |
| 3835.39 | H I | H9 | 0.237 | 3833.13 | 5.47 ± 0.67 | 3831.34 | 6.23 ± 0.50 | 3827.67 | 6.30 ± 0.44 |
| 3867.49 | He I | 20 | 0.231 | 3866.72 | 3.03 ± 0.55 | 3864.69 | 2.41 ± 0.35 | 3861.05 | 14.43 ± 0.59 |
| 3868.75 | [Ne III] | 1F | 0.230 | | | | | | |
| 3888.65 | He I | | 0.226 | 3886.78 | 17.84 ± 0.86 | 3884.75 | 18.36 ± 0.56 | 3881.21 | 19.08 ± 0.52 |
| 3889.05 | H I | H8 | 0.226 | | | | | | |
| 3967.46 | [Ne III] | 1F | 0.211 | – | – | – | – | 3959.91 | 3.83 ± 0.39 |
| 3970.07 | H I | H7 | 0.210 | 3968.38 | 9.92 ± 0.51 | 3965.85 | 15.63 ± 0.67 | 3962.59 | 15.60 ± 0.47 |
| 4026.21 | He I | 18 | 0.198 | – | – | 4022.19 | 1.91 ± 0.17 | 4018.72 | 1.75 ± 0.14 |
| 4068.60 | [S II] | 1F | 0.189 | 4067.08 | 1.18 ± 0.30 | 4064.17 | 2.05 ± 0.27 | 4061.31 | 0.68 ± 0.11 |
| 4076.35 | [S II] | 1F | 0.187 | 4075.60 | 0.77 ± 0.23 | 4072.05 | 0.48 ± 0.16 | 4069.15 | 0.40 ± 0.12 |
| 4101.74 | H I | H6 | 0.182 | 4100.29 | 23.34 ± 0.72 | 4097.32 | 26.06 ± 0.60 | 4094.32 | 25.89 ± 0.59 |
| 4267.15 | C II | 6 | 0.144 | – | – | 4262.89 | 0.47 ± 0.11 | – | – |
| 4340.47 | H I | H$\gamma$ | 0.127 | 4338.85 | 45.8 ± 1.1 | 4335.76 | 44.64 ± 0.98 | 4332.54 | 45.05 ± 0.96 |
| 4363.21 | [O III] | 2F | 0.121 | 4361.57 | 0.224 ± 0.079 | 4358.71 | 0.30 ± 0.10 | 4355.21 | 0.97 ± 0.13 |
| 4387.93 | He I | 51 | 0.115 | – | – | – | – | 4379.88 | 0.430 ± 0.086 |
| 4471.48 | He I | 14 | 0.096 | 4469.96 | 3.65 ± 0.31 | 4466.54 | 3.97 ± 0.20 | 4463.40 | 3.80 ± 0.14 |
| 4658.10 | [Fe III] | 3F | 0.050 | – | – | 4653.37 | 0.23 : | – | – |
| 4701.53 | [Fe III] | 3F | 0.039 | – | – | 4695.81 | 0.47 ± 0.10 | – | – |
| 4711.37 | [Ar IV] | 1F | 0.037 | – | – | – | – | – | – |
| 4713.14 | He I | 12 | 0.036 | – | – | 4707.89 | 0.33 ± 0.12 | 4704.56 | 0.420 ± 0.063 |
| 4861.33 | H I | H$\beta$ | 0.000 | 4859.47 | 100.0 ± 2.1 | 4855.98 | 100.0 ± 2.0 | 4852.42 | 100.0 ± 2.0 |
| 4921.93 | He I | 48 | -0.015 | 4920.24 | 1.00 ± 0.15 | 4916.58 | 1.01 ± 0.10 | 4912.95 | 0.985 ± 0.049 |
| 4958.91 | [O III] | 1F | -0.024 | 4957.00 | 36.64 ± 0.80 | 4953.48 | 35.15 ± 0.72 | 4949.82 | 82.9 ± 1.7 |
| 4985.9 | [Fe III] | 2F | -0.031 | – | – | – | – | 4976.88 | 0.221 ± 0.044 |
| 5006.84 | [O III] | 1F | -0.036 | 5004.90 | 110.0 ± 2.2 | 5001.36 | 105.2 ± 2.1 | 4997.66 | 252.5 ± 5.1 |
| 5015.68 | He I | 4 | -0.038 | 5013.70 | 2.05 ± 0.26 | 5010.23 | 2.12 ± 0.11 | 5005.96 | 2.43 ± 0.11 |
| 5197.90 | [N I] | 1F | -0.082 | 5197.05 | 1.28 ± 0.13 | 5193.30 | 1.09 ± 0.15 | 5189.52 | 0.676 ± 0.059 |
| 5200.26 | [N I] | 1F | -0.083 | | | | | | |
| 5517.71 | [Cl III] | 1F | -0.154 | 5515.32 | 3.11 : | 5511.76 | 0.462 ± 0.070 | 5507.53 | 0.418 ± 0.026 |
| 5537.88 | [Cl III] | 1F | -0.158 | – | – | 5531.82 | 0.396 ± 0.060 | 5527.77 | 0.278 ± 0.027 |
| 5754.64 | [N II] | 3F | -0.194 | 5752.57 | 0.80 ± 0.13 | 5748.26 | 0.800 ± 0.092 | 5744.14 | 0.480 ± 0.022 |
| 5875.64 | He I | 11 | -0.215 | 5873.48 | 11.84 ± 0.44 | 5869.32 | 12.00 ± 0.31 | 5864.94 | 12.02 ± 0.27 |
| 6300.30 | [O I] | 1F | -0.282 | 6296.69 | 1.93 ± 0.19 | 6293.38 | 2.41 ± 0.19 | 6287.74 | 1.20 ± 0.12 |
| 6312.10 | [S III] | 3F | -0.283 | 6308.08 | 1.26 ± 0.38 | 6305.71 | 1.04 ± 0.13 | 6299.52 | 0.99 ± 0.12 |
| 6363.78 | [O I] | 1F | -0.291 | – | – | 6357.18 | 0.82 ± 0.15 | 6352.98 | 0.48 ± 0.10 |
| 6548.03 | [N II] | 1F | -0.318 | 6544.85 | 25.2 ± 1.1 | 6540.62 | 32.2 ± 1.0 | 6535.25 | 12.85 ± 0.41 |
| 6562.82 | H I | H$\alpha$ | -0.320 | 6559.62 | 289.3 ± 8.6 | 6555.32 | 287.9 ± 8.7 | 6549.87 | 286.9 ± 7.2 |
| 6583.41 | [N II] | 1F | -0.323 | 6580.28 | 77.9 ± 2.5 | 6575.94 | 100.0 ± 3.0 | 6570.54 | 38.0 ± 1.0 |
| 6678.15 | He I | 46 | -0.336 | 6674.95 | 3.08 ± 0.25 | 6670.60 | 3.30 ± 0.22 | 6665.00 | 3.20 ± 0.14 |
| 6716.47 | [S II] | 2F | -0.342 | 6713.28 | 28.9 ± 1.2 | 6708.84 | 30.04 ± 0.96 | 6703.30 | 14.02 ± 0.45 |
| 6730.85 | [S II] | 2F | -0.344 | 6727.66 | 21.1 ± 1.1 | 6723.20 | 22.70 ± 0.73 | 6717.61 | 10.09 ± 0.33 |
| 7002.23 | O I | 21 | -0.379 | – | – | – | – | 7005.18 | 0.46 − 0.16 |
| 7065.28 | He I | 10 | -0.387 | 7064.31 | 4.71 ± 0.43 | 7059.91 | 7.34 ± 0.28 | 7052.57 | 5.44 ± 0.23 |
| 7135.78 | [Ar III] | 1F | -0.396 | 7132.53 | 6.75 ± 0.37 | 7127.84 | 8.17 ± 0.30 | 7121.71 | 8.49 ± 0.27 |
| 7281.35 | He I | 45 | -0.414 | – | – | 7273.07 | 0.430 ± 0.056 | 7266.52 | 0.360 ± 0.066 |
| 7318.39 | [O II] | 2F | -0.418 | 7317.12 | 1.26 ± 0.38 | 7311.75 | 1.47 ± 0.08 | 7305.39 | 1.540 ± 0.088 |
| 7319.99 | [O II] | 2F | -0.418 | | | | | | |
| 7329.66 | [O II] | 2F | -0.420 | 7326.54 | 0.75 ± 0.23 | 7321.87 | 1.25 ± 0.08 | 7315.43 | 1.300 ± 0.074 |
| 7330.73 | [O II] | 2F | -0.420 | | | | | | |
| 7751.10 | [Ar III] | 2F | -0.467 | 7747.37 | 0.96 ± 0.20 | 7742.23 | 1.27 ± 0.14 | 7735.65 | 1.82 ± 0.32 |
| $c(\mathrm{H}\beta)$ | | | | 0.82 ± 0.03 | | 0.44 ± 0.04 | | 0.48 ± 0.02 | |
| $F(\mathrm{H}\beta)$ ($10^{-14}$ erg cm$^{-2}$ s$^{-1}$) | | | | 0.157 ± 0.003 | | 1.95 ± 0.04 | | 1.67 ± 0.03 | |

**Table A6.** Dereddened line intensity ratios with respect to $I(\mathrm{H}\beta)$ = 100 of BA371, BA310 and BA374 of M 31.

| | | | | BA371 | | BA310 | | BA374 | |
|---|---|---|---|---|---|---|---|---|---|
| $\lambda_0$ (Å) | Ion | ID | $f(\lambda)$ | $\lambda$ (Å) | $I(\lambda)$ | $\lambda$ (Å) | $I(\lambda)$ | $\lambda$ (Å) | $I(\lambda)$ |
| 3726.03 | [O II] | 1F | 0.257 | 3718.68 | 65.7 ± 2.2 | 3718.25 | 61.9 ± 1.8 | 3718.86 | 162.7 ± 4.1 |
| 3728.82 | [O II] | 1F | 0.256 | 3721.49 | 82.0 ± 2.8 | 3721.01 | 99.2 ± 2.8 | 3721.62 | 246.5 ± 6.2 |
| 3770.63 | H I | H11 | 0.249 | 3763.66 | 3.0 : | – | – | – | – |
| 3797.90 | H I | H10 | 0.244 | 3790.57 | 5.2 ± 1.8 | – | – | 3790.71 | 6.4 ± 1.9 |
| 3835.39 | H I | H9 | 0.237 | 3827.95 | 5.6 ± 1.3 | 3827.62 | 6.0 ± 1.2 | 3828.16 | 8.8 ± 1.4 |
| 3867.49 | He I | 20 | 0.231 | 3861.30 | 19.8 ± 1.0 | 3861.04 | 3.12 ± 0.79 | 3861.60 | 7.1 ± 1.1 |
| 3868.75 | [Ne III] | 1F | 0.230 | | | | | | |
| 3888.65 | He I | | 0.226 | 3881.47 | 16.6 ± 1.2 | 3881.09 | 16.07 ± 0.97 | 3881.60 | 20.0 ± 1.5 |
| 3889.05 | H I | H8 | 0.226 | | | | | | |
| 3967.46 | [Ne III] | 1F | 0.211 | 3960.23 | 6.6 ± 1.0 | – | – | – | – |
| 3970.07 | H I | H7 | 0.210 | 3962.87 | 15.2 ± 1.1 | 3962.44 | 12.83 ± 0.67 | 3963.07 | 16.5 ± 1.0 |
| 4026.21 | He I | 18 | 0.198 | 4019.05 | 1.95 ± 0.57 | – | – | 4019.31 | 3.3 ± 1.1 |
| 4068.60 | [S II] | 1F | 0.189 | – | – | 4061.11 | 1.05 ± 0.32 | 4061.63 | 2.17 ± 0.76 |
| 4101.74 | H I | H6 | 0.182 | 4094.51 | 24.86 ± 0.85 | 4094.15 | 23.3 ± 1.2 | 4094.79 | 26.4 ± 1.3 |
| 4340.47 | H I | H$\gamma$ | 0.127 | 4332.71 | 44.9 ± 1.1 | 4332.35 | 47.9 ± 1.4 | 4332.99 | 47.7 ± 1.1 |
| 4363.21 | [O III] | 2F | 0.121 | 4355.45 | 1.56 ± 0.16 | – | – | 4355.27 | 2.08 ± 0.42 |
| 4471.48 | He I | 14 | 0.096 | 4463.52 | 3.46 ± 0.25 | 4463.23 | 4.12 ± 0.34 | 4463.91 | 5.17 ± 0.47 |
| 4711.37 | [Ar IV] | 1F | 0.037 | 4704.58 | 0.55 ± 0.17 | – | – | – | – |
| 4713.14 | He I | 12 | 0.036 | | | | | | |
| 4861.33 | H I | H$\beta$ | 0.000 | 4852.61 | 100.0 ± 2.0 | 4852.17 | 100.0 ± 2.0 | 4852.88 | 100.0 ± 2.1 |
| 4921.93 | He I | 48 | -0.015 | 4913.24 | 1.194 ± 0.092 | 4912.83 | 0.90 ± 0.22 | 4913.78 | 1.46 ± 0.39 |
| 4958.91 | [O III] | 1F | -0.024 | 4950.04 | 114.1 ± 2.3 | 4949.57 | 31.44 ± 0.75 | 4950.30 | 58.8 ± 1.3 |
| 4985.9 | [Fe III] | 2F | -0.031 | – | – | 4976.44 | 0.70 ± 0.21 | – | – |
| 5006.84 | [O III] | 1F | -0.036 | 4997.89 | 347.1 ± 7.0 | 4997.41 | 93.4 ± 1.9 | 4998.15 | 170.8 ± 3.5 |
| 5015.68 | He I | 4 | -0.038 | 5006.71 | 2.56 ± 0.19 | 5006.33 | 1.98 ± 0.30 | 5006.99 | 2.84 ± 0.54 |
| 5197.90 | [N I] | 1F | -0.082 | 5189.49 | 0.78 ± 0.18 | 5187.66 | 1.37 ± 0.22 | 5189.88 | 1.98 ± 0.48 |
| 5200.26 | [N I] | 1F | -0.083 | | | | | | |
| 5270.40 | [Fe III] | 1F | -0.111 | – | – | 5260.79 | 0.38 ± 0.09 | – | – |
| 5517.71 | [Cl III] | 1F | -0.154 | 5507.77 | 0.410 ± 0.050 | 5508.40 | 0.34 ± 0.10 | 5508.53 | 0.69 ± 0.22 |
| 5537.88 | [Cl III] | 1F | -0.158 | 5527.94 | 0.377 ± 0.057 | – | – | – | – |
| 5754.64 | [N II] | 3F | -0.194 | 5744.40 | 0.475 ± 0.063 | 5743.61 | 0.64 ± 0.19 | 5745.14 | 1.78 ± 0.44 |
| 5875.64 | He I | 11 | -0.215 | 5865.21 | 11.62 ± 0.31 | 5864.78 | 15.71 ± 0.45 | 5865.67 | 11.74 ± 0.62 |
| 6300.30 | [O I] | 1F | -0.282 | 6289.13 | 1.27 ± 0.19 | 6288.21 | 1.71 ± 0.26 | 6289.32 | 6.40 ± 0.56 |
| 6312.10 | [S III] | 3F | -0.283 | 6300.65 | 1.38 ± 0.21 | 6299.16 | – | – | – |
| 6363.78 | [O I] | 1F | -0.291 | 6352.03 | 0.61 ± 0.15 | – | – | 6352.63 | 2.23 ± 0.45 |
| 6548.03 | [N II] | 1F | -0.318 | 6535.91 | 10.48 ± 0.44 | 6536.03 | 26.4 ± 1.5 | 6536.52 | 31.10 ± 0.83 |
| 6562.82 | H I | H$\alpha$ | -0.320 | 6550.70 | 282.1 ± 8.4 | 6550.68 | 284.6 ± 8.6 | 6551.18 | 288.9 ± 7.2 |
| 6583.41 | [N II] | 1F | -0.323 | 6571.38 | 33.8 ± 1.1 | 6571.35 | 78.6 ± 2.8 | 6571.86 | 94.1 ± 2.4 |
| 6678.15 | He I | 46 | -0.336 | 6666.03 | 3.16 ± 0.19 | 6666.26 | 2.92 ± 0.24 | 6666.65 | 3.01 ± 0.43 |
| 6716.47 | [S II] | 2F | -0.342 | 6704.27 | 12.26 ± 0.46 | 6704.22 | 30.8 ± 1.3 | 6704.66 | 41.3 ± 1.1 |
| 6730.85 | [S II] | 2F | -0.344 | 6718.59 | 9.32 ± 0.35 | 6718.57 | 20.98 ± 0.91 | 6719.08 | 29.47 ± 0.78 |
| 7065.28 | He I | 10 | -0.387 | 7053.15 | 3.00 ± 0.14 | 7054.04 | 6.80 ± 0.92 | 7055.23 | 10.68 ± 0.45 |
| 7135.78 | [Ar III] | 1F | -0.396 | 7122.84 | 8.33 ± 0.33 | 7122.78 | 6.36 ± 0.50 | 7123.41 | 9.72 ± 0.43 |
| 7281.35 | He I | 45 | -0.414 | 7267.35 | 0.47 ± 0.10 | – | – | – | – |
| 7318.39 | [O II] | 2F | -0.418 | 7306.59 | 1.55 ± 0.10 | – | – | 7307.46 | 3.08 ± 0.47 |
| 7319.99 | [O II] | 2F | -0.418 | | | | | | |
| 7329.66 | [O II] | 2F | -0.420 | 7316.78 | 1.096 ± 0.076 | – | – | 7317.33 | 2.09 ± 0.32 |
| 7330.73 | [O II] | 2F | -0.420 | | | | | | |
| 7751.10 | [Ar III] | 2F | -0.467 | 7737.14 | 1.49 ± 0.45 | – | – | 7737.60 | 1.69 ± 0.29 |
| $c(\mathrm{H}\beta)$ | | | | 1.12 ± 0.03 | | 0.02± 0.03 | | 0.43 ± 0.02 | |
| $F(\mathrm{H}\beta)$ ($10^{-14}$ erg cm$^{-2}$ s$^{-1}$) | | | | 0.154± 0.003 | | 3.26 ± 0.06 | | 0.140 ± 0.003 | |
